# Supplementary material for: Thermovoltage in quantum dots with attractive interaction
Source: arXiv:2003.11146 ancillary file (2020-06-17)
Supplement: Supplementary file 1 [file SupplementaryMaterial.pdf]

# Supplementary material for: Thermovoltage in quantum dots with attractive interaction

Jens Schulenborg,[1,2] Maarten R. Wegewijs,[3,4] and Janine Splettstoesser[2]
[1)]Center for Quantum Devices, Niels Bohr Institute, University of Copenhagen, DK-2100 Copenhagen
[2)]Department of Microtechnology and Nanoscience, Chalmers University of Technology, SE-41298 Göteborg
[3)]Institute for Theory of Statistical Physics, RWTH Aachen,D-52056 Aachen
[4)]Peter Grünberg Institut and JARA, Forschungszentrum Jülich, D-52425 Jülich

(Dated: 8 June 2020)

In this supplementary material, we present results for the thermovoltage and the thermoelectric performance of a quantum dot with *real repulsive interaction*. This is of interest for comparison with the results presented in the main text for attractive quantum dots. These show unexpected effects due a mapping to a *dual repulsive model* which should not be confused with "effective repulsion" by some physical mechanism. The physical quantities discussed below have been studied in several previous publications[1–13] and we merely summarize their results in a way that facilitates direct comparison.

The system of interest here is sketched in Fig. S1. The isolated quantum dot is now described by the Hamiltonian

$$H = \tilde{\varepsilon} N + |U| N_{\uparrow} N_{\downarrow}, \tag{S1}$$

which, in contrast to Eq. (1) from the main paper, has a positive sign in the interaction of strength $|U|$. The description of the environment and the coupling to the dot is the same as in the main article. A detailed analysis of the thermovoltage of this repulsive quantum dot exploiting the fermionic duality is given in Refs. 9 and 10.

In Fig. S1(b), we show the linear response Seebeck coefficient as a function of $\varepsilon = \tilde{\varepsilon} - \mu$ for energy-independent coupling $\Gamma_{\mathrm{L,R}}$ (wideband limit). Its sawtooth shape with a zero crossing at $\varepsilon = -|U|/2$ has been known and experimentally verified a long time ago[14–17]. This characteristic shape is very different from the one of the attractive quantum dot studied in the main paper. However, also here, the sharp feature at $\varepsilon = -|U|/2$ matches with the step of the dual occupation number, see Fig. S1(c). Yet, note that in this case of repulsive interaction, the feature at $\varepsilon = -|U|/2$ as predicted from its dual attractive model is less surprising, as it coincides with the particle-hole symmetric point, in contrast to our concluding remark in the summary of the main text.

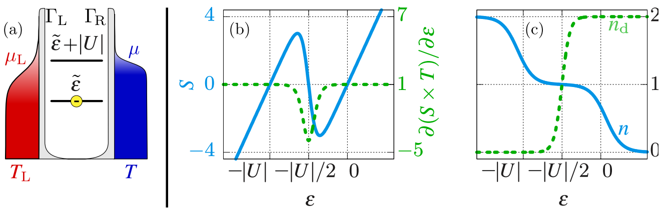


FIG. S1. (a) Sketch of quantum dot with repulsive interaction. (b) Seebeck coefficient $S$ (blue solid) and its derivative (green dashed), and (c) equilibrium charge $n$ and its dual $n_{\mathrm{d}}$, as function of dot level $\varepsilon = \tilde{\varepsilon} - \mu$. We take $T = |U|/10$ and $\Gamma_{\mathrm{L,R}}$ energy-independent.

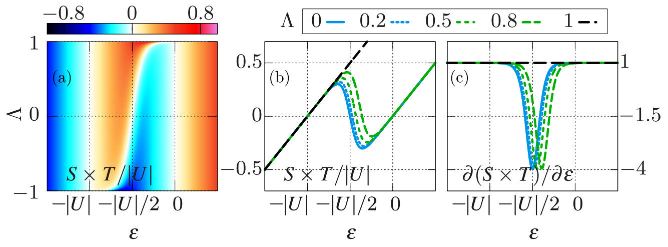


FIG. S2. Seebeck coefficient [(a) and (b)] and its derivative at fixed $\Lambda$ (c) as function of dot level $\varepsilon$ and coupling-asymmetry $\Lambda$. We take energy-dependent $\Gamma_{\mathrm{L}}(E), \Gamma_{\mathrm{R}}(E)$ and $T = |U|/10$.

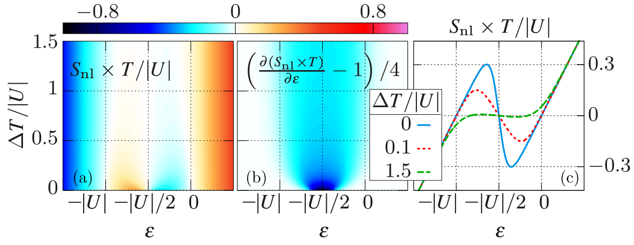


FIG. S3. Nonlinear thermovoltage [(a) and (c)] and its derivative (b) as function of dot level $\varepsilon$ and temperature gradient $\Delta T/|U|$. We take $T = |U|/10$ and $\Gamma_{\mathrm{L}}, \Gamma_{\mathrm{R}}$ energy-independent.

The $\varepsilon$-dependence of the Seebeck coefficient for energy-dependent couplings $\Gamma_{\mathrm{L,R}}(E)$ is displayed in Fig. S2. This energy-dependence has been investigated in detail in Ref. 10. The main features are the following: the central zero crossing gets shifted with larger energetic coupling asymmetry $\Lambda$ while the outer zeros around $\varepsilon = 0, -|U|$ are not affected for moderate $\Lambda$. Only for $|\Lambda| \to 1$ is the Seebeck coefficient reduced to the contribution of a single resonance. This then leads to a sole zero crossing.

Figure S3 displays the nonlinear thermovoltage as a function of dot level $\varepsilon$. This regime of nonlinear response to a large temperature difference has been discussed using duality in Ref. 9; for other studies based on different theoretical approaches, see Refs. 2, 4, 5, 7–9, and 11. Importantly, in contrast to the attractive case of the main text, the nonlinear response is qualitatively quite different from the linear response: for large $\Delta T$, the zero-crossings at $\varepsilon = 0, -|U|$ disappear and the thermovoltage in the interval $-|U| < \varepsilon < 0$ becomes flat as function of $\varepsilon$. Outside of this interval, for level positions far away from the electron-hole symmetric point, the linear

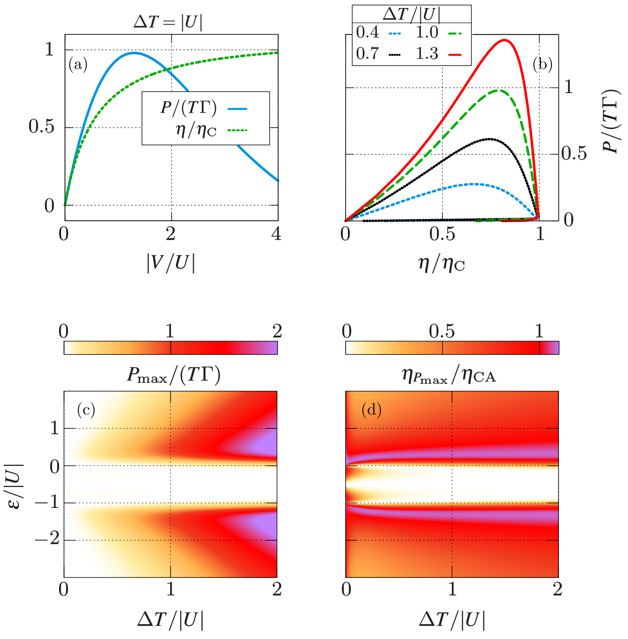


FIG. S4. (a) Power $P$ and efficiency $\eta$ as function of the voltage bias $V$ at fixed level position, $\varepsilon = 0.47|U|$, $\Delta T = |U|$, $T = |U|/10$. (b) Efficiency versus power at fixed level position, $\varepsilon = 0.47|U|$ for different temperature biases $\Delta T$. (c) Power $P_{\max}$ maximized over $V$. (d) Efficiency $\eta_{P_{\max}}$ at maximum power.

dependence on $\varepsilon$ is maintained even for large $\Delta T$.

Finally, in Fig. S4, we show plots characterizing the performance of the quantum dot as a steady state heat engine. Qualitatively, these plots are very similar to the ones discussed in the main paper for a quantum dot with attractive interaction. However, one should note the following important differences: First, we stress that due to the inverted sequence of addition energies ($\varepsilon < \varepsilon + |U|$ for repulsive vs. $\varepsilon > \varepsilon - |U|$ for attractive interaction), the level position of optimal power output is different for the two cases. At these optimal level positions, the maximum power output and the efficiency at maximum power take *larger values* for the repulsive dot compared to the attractive one. In particular, the Curzon-Ahlborn bound is exceeded in larger parameter regimes, see purple regions in Fig. S4(d). However, a different comparison concerns the *size of parameter regions* in which the device produces sizable power output. For the repulsive dot presented here, this power output is suppressed in the entire Coulomb blockade regime $-|U| < \varepsilon < 0$. This is in contrast to the attractive dot studied in the main paper, where the power is only suppressed at a sharp dip at the particle-hole symmetric point $\varepsilon = |U|/2$.

[1] M. Esposito, K. Lindenberg, and C. Van den Broeck, "Thermoelectric efficiency at maximum power in a quantum dot," EPL **85**, 60010 (2009).
[2] M. Leijnse, M. R. Wegewijs, and K. Flensberg, "Nonlinear thermoelectric properties of molecular junctions with vibrational coupling," Phys. Rev. B **82**, 045412 (2010).
[3] D. M. Kennes, D. Schuricht, and V. Meden, "Efficiency and power of a thermoelectric quantum dot device," EPL **102**, 57003 (2013).
[4] S. F. Svensson, E. A. Hoffmann, N. Nakpathomkun, P. M. Wu, H. Q. Xu, H. A. Nilsson, D. Sánchez, V. Kashcheyevs, and H. Linke, "Nonlinear thermovoltage and thermocurrent in quantum dots," New J. Phys. **15**, 105011 (2013).
[5] M. A. Sierra and D. Sánchez, "Strongly nonlinear thermovoltage and heat dissipation in interacting quantum dots," Phys. Rev. B **90**, 115313 (2014).
[6] B. Sothmann, R. Sánchez, and A. N. Jordan, "Thermoelectric energy harvesting with quantum dots," Nanotechnology **26**, 032001 (2014).
[7] A. Svilans, A. M. Burke, S. F. Svensson, M. Leijnse, and H. Linke, "Nonlinear thermoelectric response due to energy-dependent transport properties of a quantum dot," Physica E **82**, 34–38 (2016).
[8] D. Sánchez and R. López, "Nonlinear phenomena in quantum thermoelectrics and heat," C. R. Phys. **17**, 1060–1071 (2016).
[9] J. Schulenborg, A. Di Marco, J. Vanherck, M. R. Wegewijs, and J. Splettstoesser, "Thermoelectrics of Interacting Nanosystems—Exploiting Superselection Instead of Time-Reversal Symmetry," Entropy **19**, 668 (2017).
[10] J. Schulenborg, J. Splettstoesser, and M. R. Wegewijs, "Duality for open fermion systems: Energy-dependent weak coupling and quantum master equations," Phys. Rev. B **98**, 235405 (2018).
[11] P. A. Erdman, F. Mazza, R. Bosisio, G. Benenti, R. Fazio, and F. Taddei, "Thermoelectric properties of an interacting quantum dot based heat engine," Phys. Rev. B **95**, 245432 (2017).
[12] M. Josefsson, A. Svilans, A. M. Burke, E. A. Hoffmann, S. Fahlvik, C. Thelander, M. Leijnse, and H. Linke, "A quantum-dot heat engine operating close to the thermodynamic efficiency limits," Nat. Nanotechnol. **13**, 920–924 (2018).
[13] M. Josefsson, A. Svilans, H. Linke, and M. Leijnse, "Optimal power and efficiency of single quantum dot heat engines: Theory and experiment," Phys. Rev. B **99**, 235432 (2019).
[14] C. W. J. Beenakker, "Theory of Coulomb-blockade oscillations in the conductance of a quantum dot," Phys. Rev. B **44**, 1646 (1991).
[15] C. W. J. Beenakker and A. A. M. Staring, "Theory of the thermopower of a quantum dot," Phys. Rev. B **46**, 9667 (1992).
[16] A. A. M. Staring, L. W. Molenkamp, B. W. Alphenaar, H. van Houten, O. J. A. Buyk, M. A. A. Mabesoone, C. W. J. Beenakker, and C. T. Foxon, "Coulomb-Blockade Oscillations in the Thermopower of a Quantum Dot," EPL **22**, 57 (1993).
[17] A. S. Dzurak, C. G. Smith, M. Pepper, D. A. Ritchie, J. E. F. Frost, G. A. C. Jones, and D. G. Hasko, "Observation of Coulomb blockade oscillations in the thermopower of a quantum dot," Solid State Commun. **87**, 1145–1149 (1993).
